# Supplementary material for: Demo: Soccer Information Retrieval via Natural Queries using SoccerRAG
Source: arXiv:2406.01280 source file (2024-07-22)
Supplement: Supplementary file 1 [file appendix.tex]

\nobalance
\section*{Demo Requiremnets}

\begin{itemize}
    \item \textbf{Hardware:} We will transport our own equipment directly to the venue. 
    \item \textbf{Floor space and furniture:} Our setup requires a modest floor space of 4 square meters and will operate independently without the need for wall support, as it will be run on a local laptop. The exhibit setup requires one table to hold the equipment. No additional seating is required as the demonstration is designed for a standing audience.
    \item \textbf{Power:} Our power requirements are minimal, three electrical sockets (220V) are needed to accommodate all devices. 
    \item \textbf{Monitor and cables:} We require a 32-inch display for visual presentations with HDMI and power cable for it. 
    \item \textbf{Internet:} We reqire wireless Internet to be provisioned at the venue, eduroam WiFi acceptable.
    \item \textbf{Other:} We can optionally make use of a poster stand, able to accommodate a vertical A0-sized poster, along with appropriate poster pins.
\end{itemize}
